# Supplementary material for: Distance Matters in Human-Object Interaction Detection
Source: arXiv:2207.01869 source file (2022-07-05)
Supplement: Supplementary file 1 [file 6_appendix.tex]

\section{Additional Experiments}
